# Supplementary material for: Bipartite entanglement of large quantum systems
Source: arXiv:1206.6749 source file (2012-06-29)
Supplement: Supplementary file 1 [file AppendixA.pdf]

# Appendix A

## Steepest descent method

The steepest descent method is an approximation scheme to evaluate a class of contours integrals in a complex domain of the form

$$I_N = \int_C dz e^{NA(z)} \quad (\text{A.1})$$

in the large  $N$  limit, being the contour  $C$  contained within the domain of analyticity of  $A$ . The steepest descent method is an application of the Cauchy's integral theorem according to which the contour of integration can be deformed without changing  $I_N$ . If we assume that the global maximum of  $A(z)$  is not on the boundary of  $D$ , it corresponds either to a singularity of the function or to a regular point where the derivative of  $A$  vanishes,

$$A'(z) = 0. \quad (\text{A.2})$$

We will focus on the second case. A point  $z_c$  where condition (A.2) is satisfied is, in general, a *saddle point* for the curves of constant  $\text{Re}A(z)$ . In order to avoid cancellations due to the oscillatory behavior of the phase of the integrand we need to choose as contour of integration a *path of steepest descent*, that is a directed curve whose tangent at each point has a direction in which the rate of descent is maximal (*direction of steepest descent*). Indeed it can be proved that such curves are defined by

$$\text{Im}A(z) = \text{Im}A(z_c). \quad (\text{A.3})$$

Thus along this path the phase of the integrand remains constant and the leading contribution to the integral comes from a neighbourhood of  $z_c$ . If we make the change of variables

$$t = A(z_c) - A(z) \quad (\text{A.4})$$

the path of steepest descent  $C$  can be mapped onto the positive real axis:

$$I_N = e^{NA(z_c)} \int_0^{+\infty} dt \mathcal{A}(t) e^{Nt}, \quad \mathcal{A}(t) = \left. \frac{dz}{dA(z)} \right|_{z=A^{-1}(A(z_c)-t)}. \quad (\text{A.5})$$

We have assumed that the upper limit of integration can be extended to  $+\infty$  due to the fast exponential decay away from  $A(z_c)$ . By applying the Watson's lemma for  $t \rightarrow 0_+$ , in the limit  $N \rightarrow \infty$ , we find

$$I_N \simeq \sqrt{\frac{\pi}{2N|A''(z_c)|}} e^{NA(z_c)+i\theta_{1,2}} \quad (\text{A.6})$$

where  $\theta_1$  and  $\theta_2$  are the directions of steepest descent for the case  $A''(z_c) \neq 0$ , that is  $(z - z_c) = |z - z_c| e^{i\theta_i}$  for  $z \in C$  and  $1 \leq i \leq 2$ . For a more general form of integral (A.1)

$$I_N = \int_C dz g(z) e^{NA(z)} \quad (\text{A.7})$$

being  $g(z)$  an analytic function in a region of the complex plane that includes  $C$ , we have to multiply expression (A.6) by the constant factor  $g(z_c)$ . We remark that in almost cases the leading term of this general expression can be retrieved by expanding  $A$  around the maximum and approximate expression (A.1) with a Gaussian integral.

Another generalization of the above results is given by the  $n$ -dimensional integral on  $\mathbb{R}^n$

$$I_N = \int d^n z e^{NA(z_1, z_2, \dots, z_n)}. \quad (\text{A.8})$$

In the limit  $N \rightarrow \infty$  it can be shown that

$$I_N = (2\pi N)^{n/2} [\det \mathbf{A}^{(2)}]^{-1/2} e^{NA(\vec{z}_c)}, \quad (\text{A.9})$$

being  $\vec{z}_c = \{z_{c1}, \dots, z_{cn}\}$  and  $\mathbf{A}^{(2)}$  the matrix of the second partial derivatives

$$[\mathbf{A}^{(2)}]_{ij} = \frac{\partial^2 A(\vec{z}_c)}{\partial z_i \partial z_j}, \quad \forall i, j \in \{1, \dots, n\}. \quad (\text{A.10})$$
